# Supplementary material for: ConsisDrive: Identity-Preserving Driving World Models for Video Generation by Instance Mask
Source: arXiv:2602.03213 source file (2026-02-10)
Supplement: Supplementary file 2 [file control.tex]

\begin{figure}[ht]
\centering
% \begin{minipage}{\linewidth}
%     \centering
%     \includegraphics[width=\linewidth]{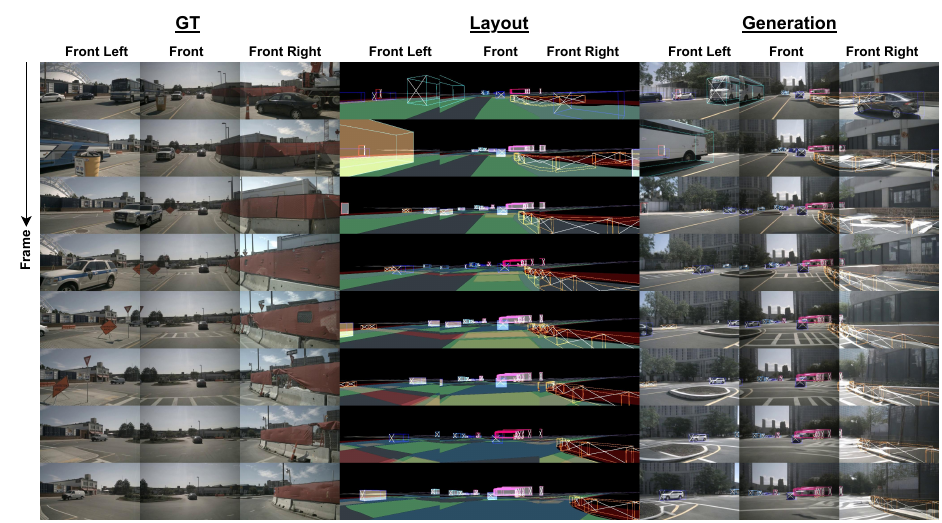} 
%     \subcaption{Relative Motion Understanding.}
%     \label{fig:subfig3}
% \end{minipage}\hfill
\begin{minipage}{\linewidth}
    \centering
    \includegraphics[width=\linewidth]{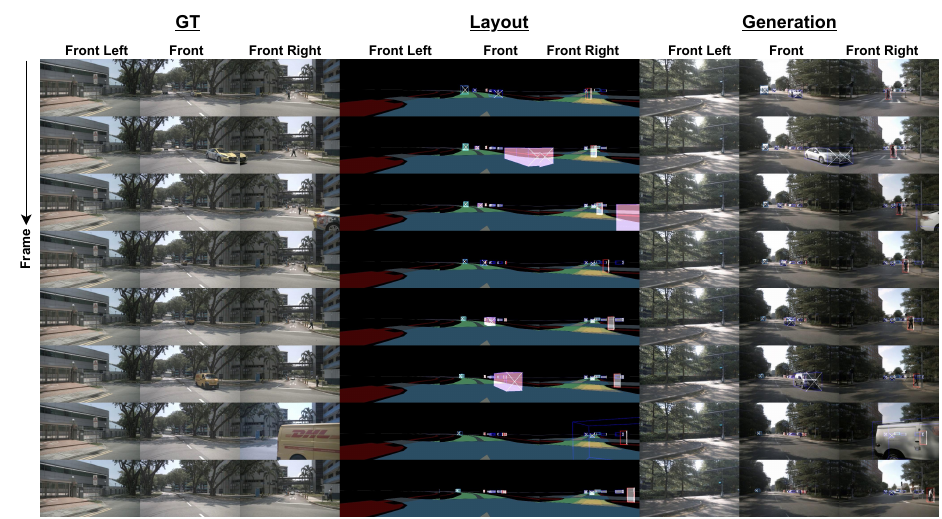} 
    \subcaption{Objects track their attributes maintaining temporal consistency.}
    \label{fig:subfig1_control}
\end{minipage}
\begin{minipage}{\linewidth}
    \centering
    \includegraphics[width=\linewidth]{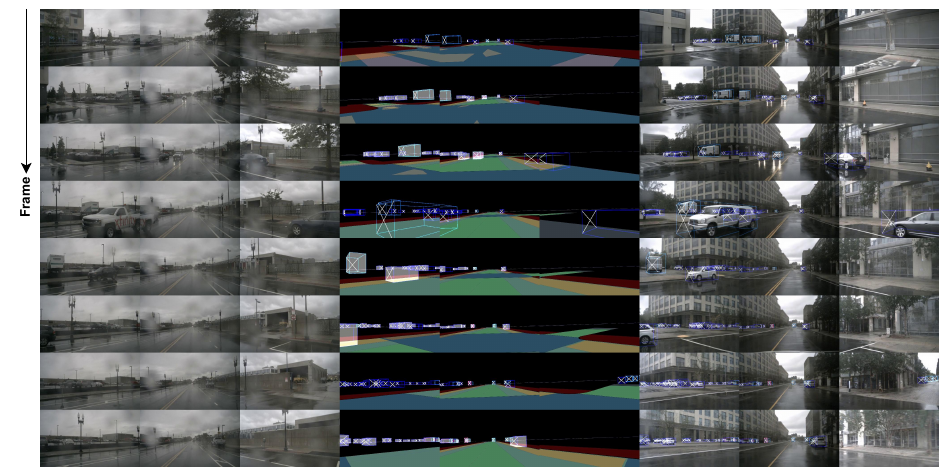} 
    \subcaption{Small and densely packed objects rendered at correct locations.}
    \label{fig:subfig2_control}
\end{minipage}
\caption{ Precise control mechanisms. We overlay the 3D bounding box projections onto the generated videos. The precision of control is reflected in: 
\textbf{(1)} Objects in the scene are accurately placed and sized to align with their \textit{projected bounding boxes}, as shown in \ref{fig:subfig1_control} and \ref{fig:subfig2_control}. 
\textbf{(2)} Drivable areas, sidewalks, and zebra crossings are faithfully generated following the \textit{road map projections}, as shown in \ref{fig:subfig1_control} and \ref{fig:subfig2_control}. 
\textbf{(3)} Objects track their previous attributes as guided by the \textit{instance flow}, ensuring temporal consistency across frames. As shown in Figure~\ref{fig:subfig1_control}, the pink-rendered instance flow directs the model to generate the white sedan, maintaining its consistent attributes over time.
\textbf{(4)} Small and densely packed objects are precisely rendered at their correct locations, following \textit{3D bounding box coordinates}, as shown in \ref{fig:subfig2_control}.
%Full-length videos are available on our project page in the supplementary materials \textcolor{red}{./drivephysica/page.html}
}
\label{fig:control}
\end{figure}
