# Supplementary material for: ConsisDrive: Identity-Preserving Driving World Models for Video Generation by Instance Mask
Source: arXiv:2602.03213 source file (2026-02-10)
Supplement: Supplementary file 3 [file X_suppl.tex]

% \clearpage
%\setcounter{page}{1}
%\maketitlesupplementary

%\appendix

\section{More Experimental Details}  
\label{app: exp}

We provide a project page for additional video results in the supplementary materials.
\textcolor{red}{Please unzip the entire supplementary materials archive before opening the webpage. Tested OK on macOS and Windows 10 systems.}

\subsection{Training Details}
\label{app: Training}
Our method is implemented based on OpenSora V2.0 \cite{peng2025opensora20trainingcommerciallevel}. 
Initially, we train for 20k iterations on the front-view videos from the NuScenes training set. 
Next, to adapt to multi-view positional encoding, we froze the backbone and fine-tuned the patch embedder for 2k iterations. 
Finally, we added all the control modules and trained the entire model for 100k iterations with a mini-batch size of 1. 
All training inputs were set to 16x256x448 and performed on 64 A100 GPUs. Additionally, during training, we set a 0.2 probability of not adding noise to the first frame and assigned a timestep of 0 to the first frame, enabling the model to have image-to-video generation capability. As a result, during testing, the model can autoregressively iterate. Experimental results show that our method can stably generate over 200 frames and the long video is included in the project webpage in the supplementary materials.

\section{Preliminary}
\label{section:preliminary}

\textbf{Latent Video Diffusion Model~(LVDM).}
The LVDM enhances the stable diffusion model ~\cite{ramesh2022hierarchical} by integrating a 3D U-Net, thereby empowering efficient video data processing. This 3D U-Net design augments each spatial convolution with an additional temporal convolution and follows each spatial attention block with a corresponding temporal attention block. It is optimized by employing a noise-prediction objective function:
\begin{equation}
    l_\epsilon = ||\epsilon - \epsilon_\theta(z_t, t, c)||^2_2,
    \label{eq:training_objective}
\end{equation}
Here, $\epsilon_\theta(\cdot)$ signifies the 3D U-Net's noise prediction function. The condition 
$c$ is guided into the U-Net using cross-attention for adjustment. Meanwhile, $z_t$ denotes the noisy hidden state, evolving like a Markov chain that progressively adds Gaussian noise to the initial latent state $z_0$:
\begin{equation}
    z_t=\sqrt{\bar{\alpha}_t}z_0 + \sqrt{1 - \bar{\alpha}_t}\epsilon, \quad\epsilon \sim \mathcal{N}(0, I),
    \label{eq:add_noise}
\end{equation}
where $\bar{\alpha}_t = \prod_{i=1}^t(1-\beta_t)$ and $\beta_t$ is a coefficient that controls the noise strength in step $t$.

\noindent \textbf{MMDiT.}
Inspired by FLUX’s MMDiT \cite{flux2024}, OpenSora V2.0 \cite{peng2025opensora20trainingcommerciallevel} employs a hybrid transformer architecture that incorporates both dual-stream and single-stream processing blocks. 
In the dual-stream blocks, text and video information are processed separately to facilitate more effective feature extraction within each modality.
Subsequently, single-stream blocks integrate these features to facilitate effective cross-modal interactions. 
To further enhance the model’s ability to capture spatial and temporal information, we apply 3D RoPE (Rotary Position Embedding), which extends traditional positional encoding to three-dimensional space, allowing the model to better represent motion dynamics across time.

For text encoding, it leverages T5-XXL \cite{chung2024scaling} and CLIP-Large \cite{Radford2021LearningTV}, two high-capacity pretrained models known for their strong semantic understanding. 
T5-XXL captures complex textual semantics,
while CLIP-Large improves alignment between text and visual concepts, leading to more accurate prompt adherence in video generation.

\section{More Quantitative Results}

\subsection{Evaluation on Planning Task.} 
% planning
\label{app:planning}
We also assess our model in the planning task in autonomous driving.
Planning task \cite{hu2023planningorientedautonomousdriving} relies on temporally coherent trajectories of surrounding agents to support accurate motion forecasting. 
Therefore, planning task performance also serves as a comprehensive indicator of instance-level temporal consistency. 

To validate our approach, we evaluate the generated nuScenes validation data using pretrained planning model UniAD \cite{shi2016uniad} in Tab.~\ref{tab:planning}.
The L2 loss and collision rates closely match the performance of the original data, demonstrating clear benefits from improved instance-level temporal consistency.

\begin{table}[tb]
    \centering
    \footnotesize
    \resizebox{0.475\textwidth}{!}{
        \setlength{\tabcolsep}{4pt}
        \begin{tabular}{c |c c c c |c c c c }
            \toprule
            \multirow{2}{*}{Eval Data} & \multicolumn{4}{c|}{L2(m)$\downarrow$} & \multicolumn{4}{c}{Col. Rate$\downarrow$} \\
            & 1s & 2s & 3s & Avg. & 1s & 2s & 3s & Avg. \\
            \hline
            Oracle & 0.48 & 0.96 & 1.65 & 1.03 & 0.0005 & 0.0017 & 0.0071 & 0.0031 \\
            \titleDef~ & 0.60 & 1.49 & 2.38 & 1.55 & 0.0020 & 0.0087 & 0.0124 & 0.0100 \\ 
            \bottomrule
        \end{tabular}
    }
    \caption{Comparison on planning task using the pre-trained planning model UniAD \cite{shi2016uniad}. 
    The L2 loss and collision rates closely match the performance of the original data, highlighting the benefits of enhanced temporal consistency.
    }
    \label{tab:planning}
\end{table}

\section{More Visualization Results}
Here, we provide additional visualization results to showcase our model's strong ability to generate high-fidelity, instance-level temporally consistent multi-view driving videos. 
We sample 8 frames from each generated video as a demo to save space in the paper. Our model is capable of generating long-duration driving videos through iterative processing. 
We provide a web page in the supplementary materials for additional results. Please refer to the webpage in the supplementary materials for visualization results.

\begin{figure}[t]
\centering
\includegraphics[width=0.8\linewidth]{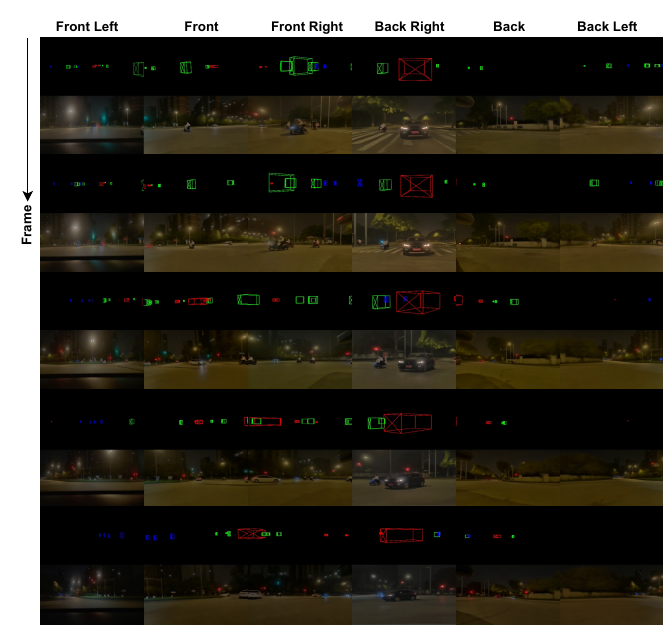} 
\caption{Results on private dataset. This demonstrates that we achieved similar generation quality as on nuScenes, highlighting the generalization capability of \titleDef.}
\label{fig:private}
\end{figure}

\subsection{Results on our private dataset}
\label{app:private data}
In addition to public datasets, we trained on a 200-hour private dataset. The results, as shown in Fig. \ref{fig:private}, demonstrate that we achieved similar generation quality as on nuScenes, highlighting the generalization capability of our method.

\section{Limitations}

Our work establishes a identity-preserving framework for generating high-quality, multi-view driving videos, achieving state-of-the-art performance in both video generation quality and downstream perception task validation. 
However, certain limitations remain, mainly due to time and resource constraints.

Future research could explore the integration of more advanced generative models, such as SD-XL ~\cite{DBLP:journals/corr/abs-2307-01952}, and develop more efficient methods to produce high-fidelity videos at larger spatial resolutions. 
Additionally, the computational cost of inference for \titleDef~ is relatively high, which presents another avenue for improvement. Enhancing the efficiency of \titleDef~ will be a key focus in future developments to make the model more practical for real-world applications.
