# Supplementary material for: ConsisDrive: Identity-Preserving Driving World Models for Video Generation by Instance Mask
Source: arXiv:2602.03213 source file (2026-02-10)
Supplement: Supplementary file 4 [file carla.tex]

\begin{figure}[ht]
\centering
\includegraphics[width=0.76\linewidth]{figures/brake2.pdf} 
\caption{\textbf{Long-tail scenarios simulation.} 
Using CARLA’s highly configurable simulation environment, we create synthetic control conditions which represent complex driving scenarios (e.g., sudden braking), and then utilize InstaDrive to generate corresponding videos.
}
\label{fig:carla}
\end{figure}
