# Supplementary material for: ConsisDrive: Identity-Preserving Driving World Models for Video Generation by Instance Mask
Source: arXiv:2602.03213 source file (2026-02-10)
Supplement: Supplementary file 5 [file noise1.tex]

\begin{figure}[ht]
\centering
\includegraphics[width=\linewidth]{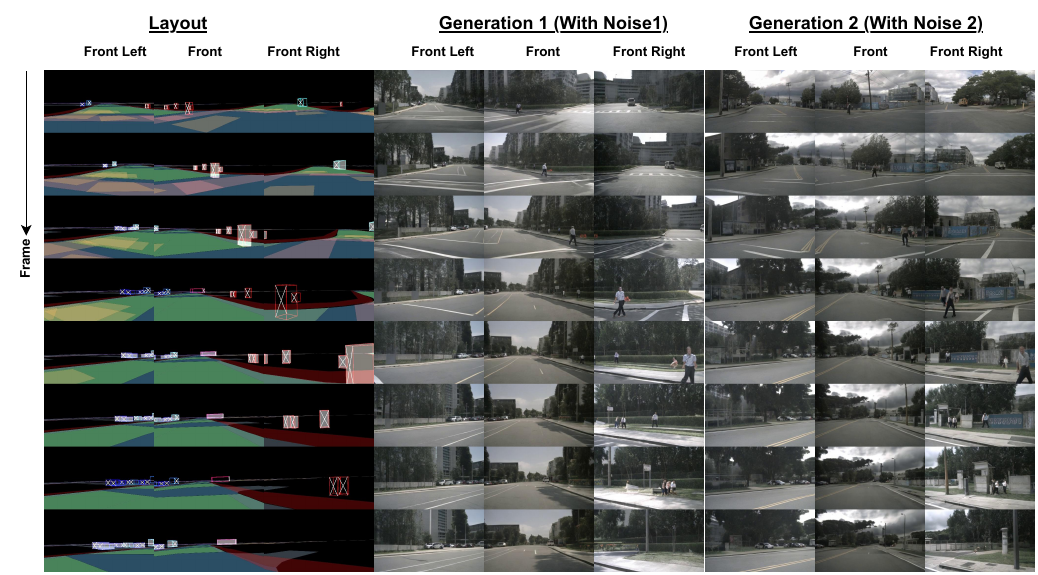} 
\caption{Diverse videos using \textbf{varying noise inputs} and \textbf{the same control conditions}. 
By introducing stochastic noise while maintaining consistent control signals—such as 3D bounding box coordinates, lane line projections, and instance flow—our model can produce a variety of videos that adhere to the defined constraints.
%Full-length videos are available on our project page in the supplementary materials \textcolor{red}{./drivephysica/page.html}
}
\label{fig:noise}
\end{figure}
