# Supplementary material for: ConsisDrive: Identity-Preserving Driving World Models for Video Generation by Instance Mask
Source: arXiv:2602.03213 source file (2026-02-10)
Supplement: Supplementary file 6 [file Appendix-experiment.tex]

\section{More Experimental Details}  
\label{app: exp}

We provide a project page for additional video results in the supplementary materials.
\textcolor{red}{Please unzip the entire supplementary materials archive before opening the webpage. Tested OK on macOS and Windows 10 systems.}

\subsection{Training Details}
\label{app: Training}
Our method is implemented based on OpenSora V2.0 \cite{peng2025opensora20trainingcommerciallevel}. 
Initially, we train for 20k iterations on the front-view videos from the NuScenes training set. 
Next, to adapt to multi-view positional encoding, we froze the backbone and fine-tuned the patch embedder for 2k iterations. 
Finally, we added all the control modules and trained the entire model for 100k iterations with a mini-batch size of 1. 
All training inputs were set to 16x256x448 and performed on 64 A100 GPUs. Additionally, during training, we set a 0.2 probability of not adding noise to the first frame and assigned a timestep of 0 to the first frame, enabling the model to have image-to-video generation capability. As a result, during testing, the model can autoregressively iterate. Experimental results show that our method can stably generate over 200 frames and the long video is included in the project webpage in the supplementary materials.
