# Supplementary material for: ConsisDrive: Identity-Preserving Driving World Models for Video Generation by Instance Mask
Source: arXiv:2602.03213 source file (2026-02-10)
Supplement: Supplementary file 7 [file Appendix-limitations.tex]

\section{Limitations}

Our work establishes a identity-preserving framework for generating high-quality, multi-view driving videos, achieving state-of-the-art performance in both video generation quality and downstream perception task validation. 
However, certain limitations remain, mainly due to time and resource constraints.

Future research could explore the integration of more advanced generative models, such as SD-XL ~\cite{DBLP:journals/corr/abs-2307-01952}, and develop more efficient methods to produce high-fidelity videos at larger spatial resolutions. 
Additionally, the computational cost of inference for \titleDef~ is relatively high, which presents another avenue for improvement. Enhancing the efficiency of \titleDef~ will be a key focus in future developments to make the model more practical for real-world applications.
