# Supplementary material for: ConsisDrive: Identity-Preserving Driving World Models for Video Generation by Instance Mask
Source: arXiv:2602.03213 source file (2026-02-10)
Supplement: Supplementary file 9 [file Appendix-result.tex]

\section{More Quantitative Results}

\subsection{Evaluation on Planning Task.} 
% planning
\label{app:planning}
We also assess our model in the planning task in autonomous driving.
Planning task \cite{hu2023planningorientedautonomousdriving} relies on temporally coherent trajectories of surrounding agents to support accurate motion forecasting. 
Therefore, planning task performance also serves as a comprehensive indicator of instance-level temporal consistency. 

To validate our approach, we evaluate the generated nuScenes validation data using pretrained planning model UniAD \cite{shi2016uniad} in Tab.~\ref{tab:planning}.
The L2 loss and collision rates closely match the performance of the original data, demonstrating clear benefits from improved instance-level temporal consistency.

\begin{table}[tb]
    \centering
    \footnotesize
    \resizebox{0.475\textwidth}{!}{
        \setlength{\tabcolsep}{4pt}
        \begin{tabular}{c |c c c c |c c c c }
            \toprule
            \multirow{2}{*}{Eval Data} & \multicolumn{4}{c|}{L2(m)$\downarrow$} & \multicolumn{4}{c}{Col. Rate$\downarrow$} \\
            & 1s & 2s & 3s & Avg. & 1s & 2s & 3s & Avg. \\
            \hline
            Oracle & 0.48 & 0.96 & 1.65 & 1.03 & 0.0005 & 0.0017 & 0.0071 & 0.0031 \\
            \titleDef~ & 0.60 & 1.49 & 2.38 & 1.55 & 0.0020 & 0.0087 & 0.0124 & 0.0100 \\ 
            \bottomrule
        \end{tabular}
    }
    \caption{Comparison on planning task using the pre-trained planning model UniAD \cite{shi2016uniad}. 
    The L2 loss and collision rates closely match the performance of the original data, highlighting the benefits of enhanced temporal consistency.
    }
    \label{tab:planning}
\end{table}

\section{More Visualization Results}
Here, we provide additional visualization results to showcase our model's strong ability to generate high-fidelity, instance-level temporally consistent multi-view driving videos. 
We sample 8 frames from each generated video as a demo to save space in the paper. Our model is capable of generating long-duration driving videos through iterative processing. 
We provide a web page in the supplementary materials for additional results. Please refer to the webpage in the supplementary materials for visualization results.

\begin{figure}[t]
\centering
\includegraphics[width=0.8\linewidth]{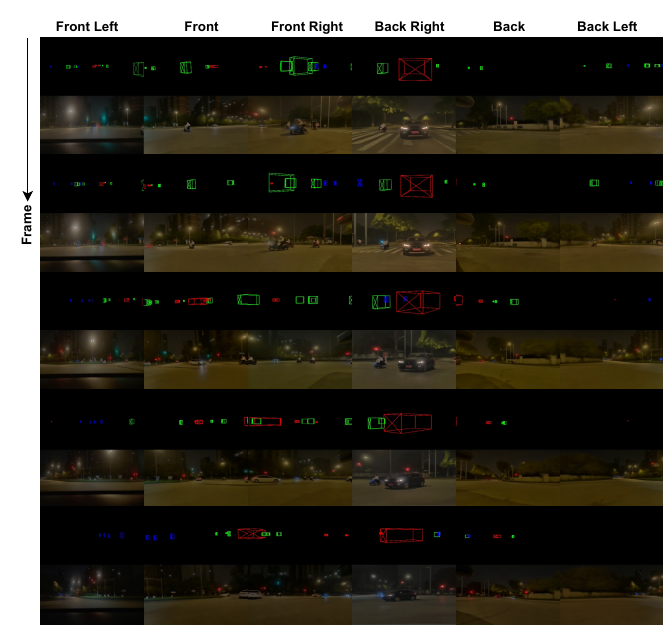} 
\caption{Results on private dataset. This demonstrates that we achieved similar generation quality as on nuScenes, highlighting the generalization capability of \titleDef.}
\label{fig:private}
\end{figure}

\subsection{Results on our private dataset}
\label{app:private data}
In addition to public datasets, we trained on a 200-hour private dataset. The results, as shown in Fig. \ref{fig:private}, demonstrate that we achieved similar generation quality as on nuScenes, highlighting the generalization capability of our method.
