# Supplementary material for: ConsisDrive: Identity-Preserving Driving World Models for Video Generation by Instance Mask
Source: arXiv:2602.03213 source file (2026-02-10)
Supplement: Supplementary file 10 [file X_suppl_new_after_rebuttal.tex]

\section{Backbone Model Generalization From Opensora to Wan}
The proposed Instance-Masked Attention and Loss are plug-and-play modules that can be inserted into any diffusion transformer with spatiotemporal attention. 
These components do not rely on any architectural details specific to OpenSora V2.0; 
instead, they target structural limitations that broadly exist across modern video diffusion transformers, including Wan 2.1/2.2:
(i) the absence of explicit instance identity conditioning, 
(ii) instance-agnostic self-attention leading to cross-instance information leakage, and 
(iii) uniform per-pixel diffusion losses that dilute foreground gradients.

To validate compatibility, we conducted an experiment by integrating the Instance-Masked Attention and Instance-Masked Loss modules into a \textbf{Wan~2.1 + ControlNet} pipeline in Fig.\ref{fig:wan}. 
The baseline Wan~2.1 + ControlNet (without ConsisDrive) still exhibits significant identity drift in Fig.\ref{fig:wan} (a), 
despite Wan's strong base modeling capability. 
This behavior is expected: Wan's transformer blocks employ the same full self-attention mechanism 
as the MMDiT architecture in OpenSora V2.0,
and therefore inherit the same intrinsic limitations regarding instance-level temporal consistency.
After plugging in our identity and trajectory masks in Fig.\ref{fig:wan} (b), the system achieves noticeably improved instance consistency across frames.
These results confirm that ConsisDrive  can be readily applied to Wan~2.1/2.2 or future foundation models.




\begin{figure}[ht]
\centering
\includegraphics[width=0.7\linewidth]{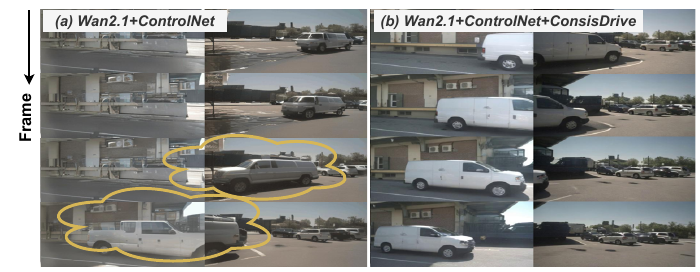} 
\caption{Backbone Model Generalization to Wan~2.1. 
\textbf{(a)} The baseline Wan~2.1 + ControlNet (without ConsisDrive) still exhibits significant identity shift in the white car's shape.
\textbf{(b)} After plugging in our Instance-Masked Attention and Instance-Masked Loss modules, the system achieves noticeably improved instance consistency across frames.}
\label{fig:wan}
\vspace{-0.5cm}
\end{figure}




\section{More Results}




\subsection{Challenges for Occlusion in Non-Continuous Trajectory}

\textbf{Method:} Instance-Masked Attention ensures consistent instance identity even when objects are occluded and reappear, the principle is demonstrated in Fig.~\ref{fig: main} (c). 
When an object (e.g., object 1) becomes occluded at frame $t+1$ and reappears at frame $t+2$, the Indicator function $I(v_k)$ tracks the object's presence across frames. At frame $t$, $1 \in I(v_0)$ when the object is visible. At frame $t+1$, the object is occluded, and at frame $t+2$, $1 \in I(v_4)$ when the object reappears.
To ensure correct feature propagation, we set $M(0, 4) = 0$ in the Instance Trajectory Mask, allowing attention between token $v_0$ and $v_4$. This enables the reliable propagation of instance-specific features across their trajectory, even after occlusion.

\textbf{Qualitative results} demonstrating our method’s handling of non-continuous trajectories are shown in Fig.~\ref{fig:Non-Continuous}, where the car maintains its identity despite temporary occlusion.

\begin{figure}[ht]
\centering
\includegraphics[width=0.5\linewidth]{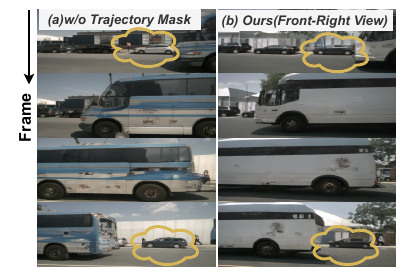} 
\caption{Challenges for Non-Continuous Trajectory. 
\textbf{(a)} Without the Trajectory Mask in the Instance-Masked Attention module, the car is occluded and reappears, but its color changes from white to black.
\textbf{(b)} With our Instance-Masked Attention, the car preserves its identity and features even after occlusion and reappearance.}
\label{fig:Non-Continuous}
%\vspace{-0.5cm}
\end{figure}






\subsection{Validation Performance on MOT}

We directly evaluate both the real validation dataset and the generated validation set of nuScenes on the Multi-Object Tracking (MOT) task, using the pretrained StreamPETR model with the same setup as in Tab. \ref{tab:perception}.  
As shown in Tab. \ref{tab: mot_val}, the validation set generated by our model achieves a relative performance of $87.5\%$ on the AMOTA metric, with only a slight increase of $5.7\%$ in the IDS metric compared to the real validation set. This demonstrates our model’s ability to propagate instance attributes across frames and confirms that the generated videos perform comparably to real data.


\begin{table}[t]
    \centering
    \footnotesize
    \resizebox{0.47\textwidth}{!}{
    \setlength{\tabcolsep}{4pt}
    \begin{tabular}{lcccccc}
        \toprule
        Method & Real & Gen. & AMOTA$\uparrow$ & AMOTP$\downarrow$ & IDS$\downarrow$  \\
        \hline
        Oracle & $\checkmark$  & - & 0.289 & 1.419 & 687 \\
        DriveDreamer2 & - & $\checkmark$   & 0.207\textcolor{blue}{(71.6\%)}   & 1.682\textcolor{blue}{(+18.5\%)} & 784 \textcolor{blue}{(+14.1\%)}  \\
        \rowcolor[gray]{.9} 
        \titleDef~ (Ours) & - & $\checkmark$   & 0.253\textcolor{blue}{(87.5\%)}    & 1.506\textcolor{blue}{(+6.1\%)} & 726 \textcolor{blue}{(+5.7\%)}\\
        \bottomrule
    \end{tabular}
    }
    \caption{Comparison of MOT task performance on real or generated nuScenes (T+I)2V validation data. Evaluated with pre-trained StreamPETR, our model outperforms DriveDreamer2, showing its ability to faithfully propagate instance attributes over frames.
    }
    \label{tab: mot_val}
\end{table}








\subsection{Ablation on Probabilistic Dynamic Masking in Instance-Masked Loss}
We set the probability $\alpha=0.5$ in the Instance-Masked Loss, meaning there is a $50\%$ chance of using the dynamic mask loss (focusing on foreground regions) and a $50\%$ chance of using the original loss (considering the entire global scene) during training.
In Sec.~\ref{sec: ablation}, we evaluate the necessity of the Instance-Masked Loss by setting $\alpha = 0$ (i.e., without IML). The results are as follows: qualitative results are presented in Fig.~\ref{fig:ablation_compare}, and quantitative results are provided in Tab.~\ref{tab: ablation}.
We have also added ablation studies on the impact of $\alpha$ in Tab.~\ref{tab:alpha}.
When $\alpha = 0$, the model is forced to equally consider both foreground and background, but background noise interferes with training, leading to a decrease in foreground consistency. 
On the other hand, as $\alpha$ approaches 1, the model excessively focuses on foreground objects, potentially losing the ability to generate coherent background content.
The complete ConsisDrive, integrating all components, yields optimal performance.





\begin{table}[htbp]
    \centering
    \footnotesize
        \centering
        \resizebox{0.475\textwidth}{!}{
        \setlength{\tabcolsep}{4pt}
        \begin{tabular}{lcccc}
            \toprule
            Settings       & FVD$\downarrow$ & FID$\downarrow$ & NDS$\uparrow$ & IDS$\downarrow$ \\
            %\hline
            %Oracle    & - & - & 46.90 & 1037\\ 
            \hline
            w/o IML($\alpha=0$) & 23.06 \textcolor{blue}{(+2.50)}& 2.69 \textcolor{blue}{(+0.43)} & 40.86 \textcolor{blue}{(-4.80)} & 596 \textcolor{blue}{(+120)}\\
            \hline
            \rowcolor[gray]{.9} 
            \titleDef~ ($\alpha=0.5$)  & 20.56 & 2.26 & 45.66 & 476\\
            \hline
            $\alpha=0.8$ & 28.13 \textcolor{blue}{(+7.57)}& 3.23 \textcolor{blue}{(+0.97)} & 35.63 \textcolor{blue}{(-10.03)} & 638 \textcolor{blue}{(+162)}\\ 
            $\alpha=1$ & 30.06 \textcolor{blue}{(+9.50)}& 5.89 \textcolor{blue}{(+3.63)} & 32.72 \textcolor{blue}{(-12.94)} & 725 \textcolor{blue}{(+249)}\\ 
            \bottomrule
        \end{tabular}
        }
        \caption{Ablation study results on Probabilistic Dynamic Masking in Instance-Masked Loss.}
        \label{tab:alpha}
\end{table}
